# Supplementary material for: PLADE-Net: Towards Pixel-Level Accuracy for Self-Supervised Single-View Depth Estimation with Neural Positional Encoding and Distilled Matting Loss
Source: arXiv:2103.07362 source file (2021-03-12)
Supplement: Supplementary file 1 [file table_supp.tex]

\begin{tabular}{clccccccccccc}
\hline
Ref & Methods & PP & Sup & Data & \#Par & abs rel\cellcolor{c_lowbest} & sq rel\cellcolor{c_lowbest}  & rmse\cellcolor{c_lowbest}  & rmse$_{\text{log}}$\cellcolor{c_lowbest}  & $\delta^1$\cellcolor{c_highbest} & $\delta^2$\cellcolor{c_highbest} & $\delta^3$\cellcolor{c_highbest} \\ 
\hline

\rowcolor{c_data}
\multicolumn{13}{c}{Improved Eigen Test Split \cite{kitti_official}}\\

our & PLADE-Net without PE & & S & K+CS & 15 & 0.075 & 0.317 & 2.990 & 0.111 & 0.938 & 0.989 & 0.997 \\
our & PLADE-Net with \cite{attentionall}'s PE & & S & K+CS & 15 & \textbf{0.070} & 0.298 & 3.100 & 0.111 & 0.935 & 0.989 & \textbf{0.998} \\
our & PLADE-Net (narrow)  & & S & K+CS & 10 & \underline{0.072} & 0.308 & 3.064 & 0.112 & 0.936 & \underline{0.990} & \textbf{0.998}\\
our & PLADE-Net (wide)   & & S & K+CS & 29 & \textbf{0.070} & \underline{0.295} & \underline{2.961} & \underline{0.108} & \underline{0.941} & \textbf{0.991} & \textbf{0.998} \\

\hline
our & PLADE-Net & & S & K+CS & 15 & \textbf{0.070} & \textbf{0.291} & \textbf{2.910} & \textbf{0.107} & \textbf{0.942} & \underline{0.990} & \textbf{0.998} \\
\hline

\end{tabular}
